# Supplementary material for: High-Dimensional Bayesian Optimization Using Both Random and Supervised Embeddings
Source: arXiv:2502.00854 source file (2025-02-02)
Supplement: Supplementary file 1 [file appendix.tex]

\section{Appendix: review on PLS and MGP methods}

In this section, a recall on PLS and MGP is provided. More details can be found in \cite{hellandStructurePartialLeast1988,GarnettActiveLearningLinear2014}.

\subsection{Partial least squares (PLS) based method:}

The PLS~\cite{hellandStructurePartialLeast1988} method searches for the most important $d_e$ orthonormal directions $\bm{a}_{(i)} \in \mathbb{R}^d$, $i \in \{1,\ldots,d_e\}$ of $\Omega$ in regards of the influence of the inputs \mbox{$\bm{X}^{(l)}_{(0)} = \left[\left[\x^{(0)}\right]^\top,\ldots,\left[\x^{(l)}\right]^\top \right]^\top \in \mathbb{R}^{d \times l}$} on the outputs $\bm{Y}^{(l)}_{s,(0)} = \bm{Y}^{(l)}_s \in \mathbb{R}^l$.
These directions are recursively defined as follows: 
\begin{gather}
	\bm{a}'_{(i)} \in \arg \max_{\bm{a}' \in \mathbb{R}^d} \left\{ \bm{a}'^\top \left[\bm{X}^{(l)}_{(i)}\right]^\top \bm{Y}^{(l)}_{s,(i)} \left[\bm{Y}^{(l)}_{s,(i)}\right]^\top \bm{X}^{(l)}_{(i)} \bm{a}' \ , \ \bm{a}'^\top \bm{a}' = 1 \right\}, \label{eq:kpls_opt}\\
	\bm{t}_{(i)} = \bm{X}^{(l)}_{(i)} \bm{a}'_{(i)}, \quad
	\bm{p}_{(i)} = \left[\bm{X}^{(l)}_{(i)}\right]^\top \bm{t}_{(i)} , \quad c_{(i)} = \left[\bm{Y}^{(l)}_{s,(i)}\right]^\top \bm{t}_{(i)} \\ \bm{X}^{(l)}_{(i+1)} = \bm{X}^{(l)}_{(i)} - \bm{t}_{(i)} \bm{p}_{(i)}, \quad
	\bm{Y}^{(l)}_{s,(i+1)} = \bm{Y}^{(l)}_{s,(i)} - c_{(i)} \bm{t}_{(i)}, \\
	\A' = [\bm{a}'_{(1)},\ldots,\bm{a}'_{(d_e)}], \quad
	\bm{P} = [\bm{p}'_{(1)},\ldots,\bm{p}'_{(d_e)}], \quad
	\A = \A' (\bm{P}^\top \A')^{-1},
\end{gather}
where $\bm{X}^{(l)}_{(i+1)} \in \mathbb{R}^{d \times l}$ and $\bm{Y}^{(l)}_{s,(i+1)} \in \mathbb{R}^d$ are the residuals of the projection of $\bm{X}^{(l)}_{(i)}$ and $\bm{Y}^{(l)}_{s,(i)}$ on the $\text{i}^{\text{th}}$ principal component $\bm{t}_{(i)} \in \mathbb{R}^d$.
Finally, $\bm{p}_{(i)} \in \mathbb{R}^d$ and $c_{(i)} \in \mathbb{R}$ are respectively the regression coefficients of $\bm{X}^{(l)}_{(i)}$ and $\bm{Y}^{(l)}_{s,(i)}$ on the $\text{i}^{\text{th}}$ principal component $\bm{t}_{(i)}$ for $i \in \{1,\ldots,d_e\}$.
In fact, the square of the covariance between $\bm{a}'_{(i)}$ and $\left[\bm{X}^{(l)}_{(i)}\right]^\top \bm{Y}^{(l)}_{s,(i)}$ is recursively maximized.

\subsection{Marginal Gaussian process (MGP) based method:}

With the MGP~\cite{GarnettActiveLearningLinear2014}, the vectored  matrix\ $\vect(\A) \in \mathbb{R}^{d \cdot d_e}$ is considered to be a realization of a Gaussian distribution \linebreak \mbox{$\mathbb{P}(A) = \mathcal{N}\left(\vect\left(\A_p\right), \bm{\Sigma}_p \right)$} where $\vect\left(\A_p\right)$ and $\bm{\Sigma}_p$ are respectively the prior mean and the covariance matrix.
The density function of $\mathbb{P}(A)$ is noted $p(\A)$.
Then, the posterior probability law of $\vect(\A)$ with respect to $\mathcal{D}_s^{(l)}$, $\mathbb{P}\left(\A | \mathcal{D}_s^{(l)}\right)$, is estimated with the following Laplace approximation:
\begin{gather}
   \mathbb{P}\left(\A | \mathcal{D}_s^{(l)}\right) \approx \mathcal{N}\left( \vect(\hat{\A}), \hat{\bm{\Sigma}} \right), \label{eq:mat_distrib} \\
    p\left(\A | \mathcal{D}_s^{(l)}\right) \approx p(\A) \cdot \mathcal{L}\left(\bm{Y}_s^{(l)},\A\right),
\end{gather}
where $\vect\left(\hat{\A}\right)$ is a local maximum of $p\left(\A | \mathcal{D}_s^{(l)}\right)$, the density function of $\mathbb{P}\left(\A | \mathcal{D}_s^{(l)}\right)$ and $\mathcal{L}$ the likelihood.
The covariance matrix $\hat{\bm{\Sigma}}$ is estimated by the inverse of the logarithm of $p\left(\A | \mathcal{D}_s^{(l)}\right)$ Hessian  matrix evaluated at $\vect\left(\hat{\A}\right)$
\begin{equation}
    \begin{split}
            \hat{\bm{\Sigma}}^{-1} & = \left.- \nabla^2 \log p\left(\A | \mathcal{D}_s^{(l)}\right)\right|_{\A=\hat{\A}} \\
             & \approx - \left. \nabla^2 \log \mathcal{L}\left(\bm{Y}_s^{(l)},\A\right) \right|_{\A=\hat{\A}} - \left. \nabla^2 \log p\left(\A\right) \right|_{\A=\hat{\A}}
    \end{split}
    \label{eq:sigma_gmp}
\end{equation}
where $\nabla^2$ is the Hessian operator with respect to $\vect(\A)$.
Although the derivatives and Hessian of the log prior are trivial, the log likelihood ones are not and are provided in~\citet{GarnettActiveLearningLinear2014} work.
The remaining details on the MGP construction are not necessary to understand the definition of the transfer matrix.
In this way, they are not introduced but can be found in~\citet{GarnettActiveLearningLinear2014}. 
In fact, the transfer matrix used when referring to the MGP dimension reduction method is given by $\hat{\A}$.
